# Supplementary material for: The role of viscosity contrast on plume structure in laboratory modeling of mantle convection
Source: arXiv:1610.09352 ancillary file (2016-10-28)
Supplement: Supplementary file 1 [file Prakash_supplementary.pdf]

The role of viscosity contrast on plume structure in laboratory modeling of mantle convection

by

Vivek N. Prakash, K. R. Sreenivas, and Jaywant H. Arakeri

# Supplementary Material

## 1 Plume spacing calculation procedure

We have seen that the planform plume structures at different $U$ have random orientations and locations, along with differences in morphology. Quantifying the plume spacing (hereafter referred to as $\lambda$) and thickness ($\eta$) from the raw images is hence a non-trivial task. An autocorrelation-based image analysis procedure has been adopted to quantify the plume spacing and plume thickness from the planform images at different $U$.

In this procedure, A Matlab code first reads a raw image and uses the adaptive histogram equalization technique in the image processing toolbox in Matlab. This is an important step as the raw images from the experiment generally have a non-uniform intensity, and also have lines caused due to a lensing effect by small plumes. These irregularities in the raw image pose problems for conversion to a binary image. We carefully convert the images into binary ensuring that all the major features of the raw image are retained. From the binary image, the code calculates an autocorrelation of each row (or column) (hereafter referred to as a line) of the image in both horizontal and vertical directions. The autocorrelation is computed using fast fourier transforms, for each line. The result is a plot with a prominent central autocorrelation peak and other neighboring peaks (which have lesser magnitudes on y-axis), and the x-axis gives the length scale. The plot is symmetric about the central peak, and the distance between the central peak and the centre of the next largest peak is the value of characteristic plume spacing in that line. Half of the thickness of the central autocorrelation peak gives the value of the thickness of the plumes. The code thus outputs a value of the characteristic plume spacing, $\lambda$, and plume thickness, $w$, for every line.

Figure 1 shows a binary image of the near-wall planform corresponding the case of $U = 1$. The length scales of $\lambda$ and $w$, obtained from the code are listed on the right side (along with the frequency of their occurence), and the length scales of $\lambda$ are indicated (to scale) in the binary image. The code picks up many different spacing values and end result is a wide distribution of spacings. The horizontal and vertical line distributions of plume spacing are added up to give a combined histogram as shown in Figure 2(a). Here, we have removed jitters in the peaks to obtain a smooth curve fit on the distribution to identify the most characteristic spacing value. This is done by taking a fourier transform of the distribution curve, the higher wavenumbers corresponding to jitters are cut-off in frequency space. This smoothening process results in a spurious peak at the end, which is ignored. In the histogram shown in Figure 2(a), the characteristic spacing values (also in the table of Figure 1) are identified as 0.4 cm with a frequency of 130, 0.77cm (frequency of 50) and so on. The plume thickness is also determined in a similar manner. The code outputs a histogram of the plume

thickness obtained from autocorrelations of horizontal (Figure 2(b)) and vertical lines of the image. Like the plume spacings, the thickness histograms from horizontal and vertical line autocorrelations are added up to give a joint histogram as shown in Figure 2(c).

In each experiment, there are typically 3-5 characteristic values (peaks) of the plume spacing and thickness (see for example, Figure 2(b)). We calculate a weighted average (with weights being the frequency of occurrence in the distribution) to identify a characteristic single value of spacing and thickness for each case of U. The weighted average is defined as: $\lambda_w = \Sigma_i \lambda_i f_i / \Sigma_i f_i$, where $\lambda_i$ is a plume spacing value and $f_i$ is its corresponding frequency of occurence (A table on page 57 of Ref (26) lists these values). The weighted average is found to be the most suitable quantity to arrive at a single characteristic spacing length scale for each case of $U$. Usage of the mode results in a bias towards smaller plume-spacing length-scales.

We compare the performance of this autocorrelation procedure with a manual inspection method. In the manual inspection, we have determined the plume spacing and thickness by careful manual mouse-clicks on the plumes in the different binary images in Matlab, and then take the value averaged over a number samples to obtain $\lambda$ and $w$. These results are also shown in Figure 3. We observe that both methods capture the same trend: both the plume spacing and thickness are a minimum at $U = 1$, and increase as $U$ moves away from one (Figure 3).

The autocorrelation method was developed to remove the subjectivity inherent in the inspection method and to have a robust method independent of the operator. But, the autocorrelation method can also pick up spurious length scales owing to reasons like the random orientations and locations of plumes. In Figure 3, in general, the autocorrelation method over-estimates $\lambda$, except when $U > 470$, and it under-estimates $w$, except for $U$ values close to 1. The autocorrelation code takes random cuts across the cross-sections of the plumes, and evaluates the chord lengths in addition to the diameter. This is the reason for its underestimation of $w$ in general, and $\lambda$ values for $U > 470$. Experiments using a larger test-section of the setup, with more number of plume structures on the mesh, especially for $U > 470$, will lead to a better estimation of plume spacing. However, note that both methods (autocorrelation and manual inspection methods) yield the same trend and agree over a wide range of $U$.

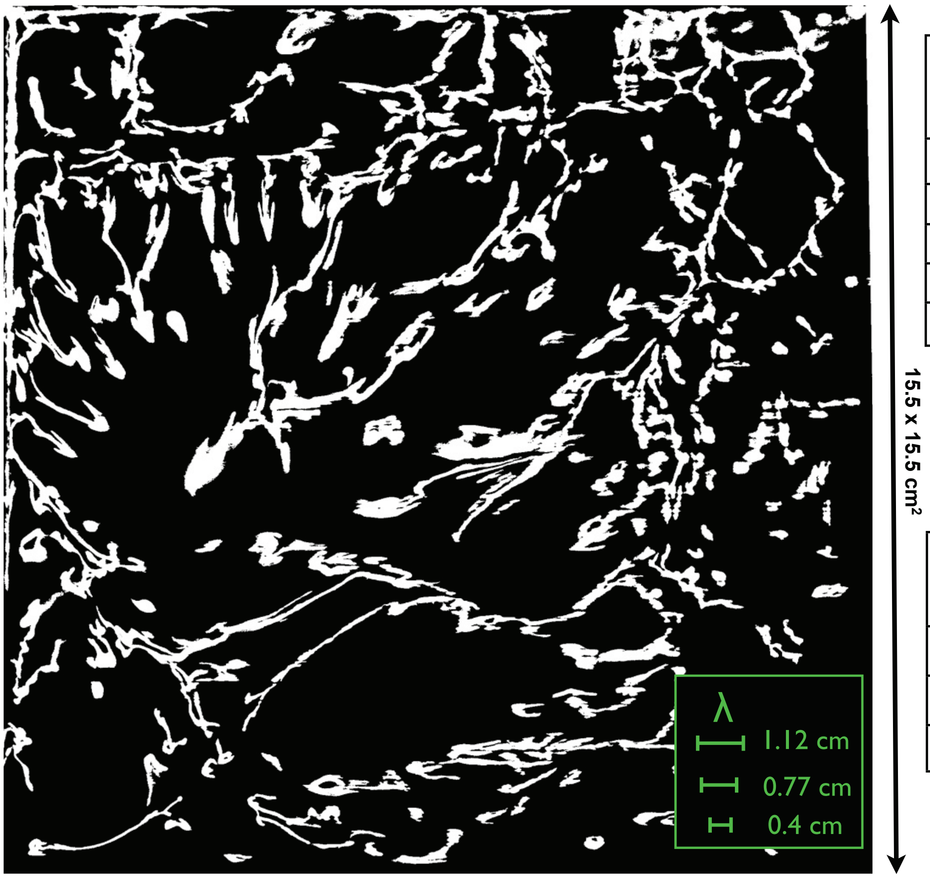


| Spacing (cm) λ | Frequency of occurrence |
|---|---|
| 0.44 | 130 |
| 0.77 | 50 |
| 1.12 | 40 |
| 2.85 | 32 |
| 4.8 | 32 |

| Thickness (cm) w | Frequency of occurrence |
|---|---|
| 0.26 | 430 |
| 0.57 | 60 |
| 0.46 | 40 |

Figure 1: The near-wall planform binary image corresponding to the case $U = 1$. The test section length scale of 15.15 cm is also shown. The tables on the right indicate the length scales corresponding to the typical plume spacings ($\lambda$) and thickness ($w$), along with their frequencies.

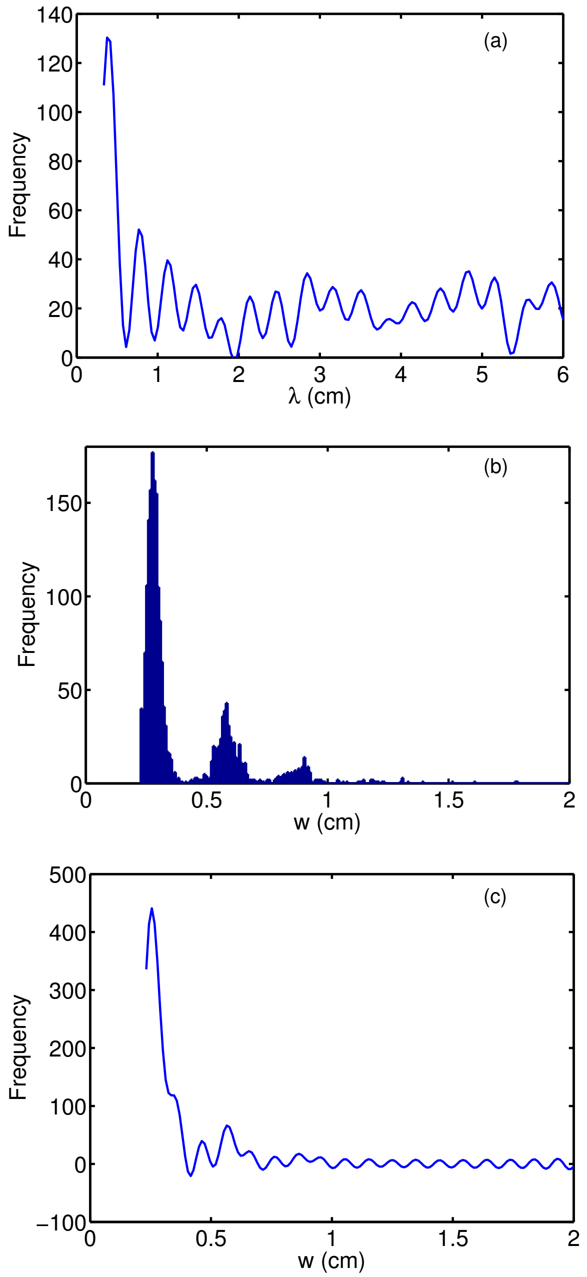


Figure 2: Histograms of characteristic plume length scales obtained from the code. (a) Plume spacings $\lambda$ - combined histogram obtained from autocorrelations of horizontal and vertical lines of the image. (b) Plume thickness $w$ - autocorrelations of horizontal lines of the image. (c) combined distributions of $w$ obtained from autocorrelations of horizontal and vertical lines of the image

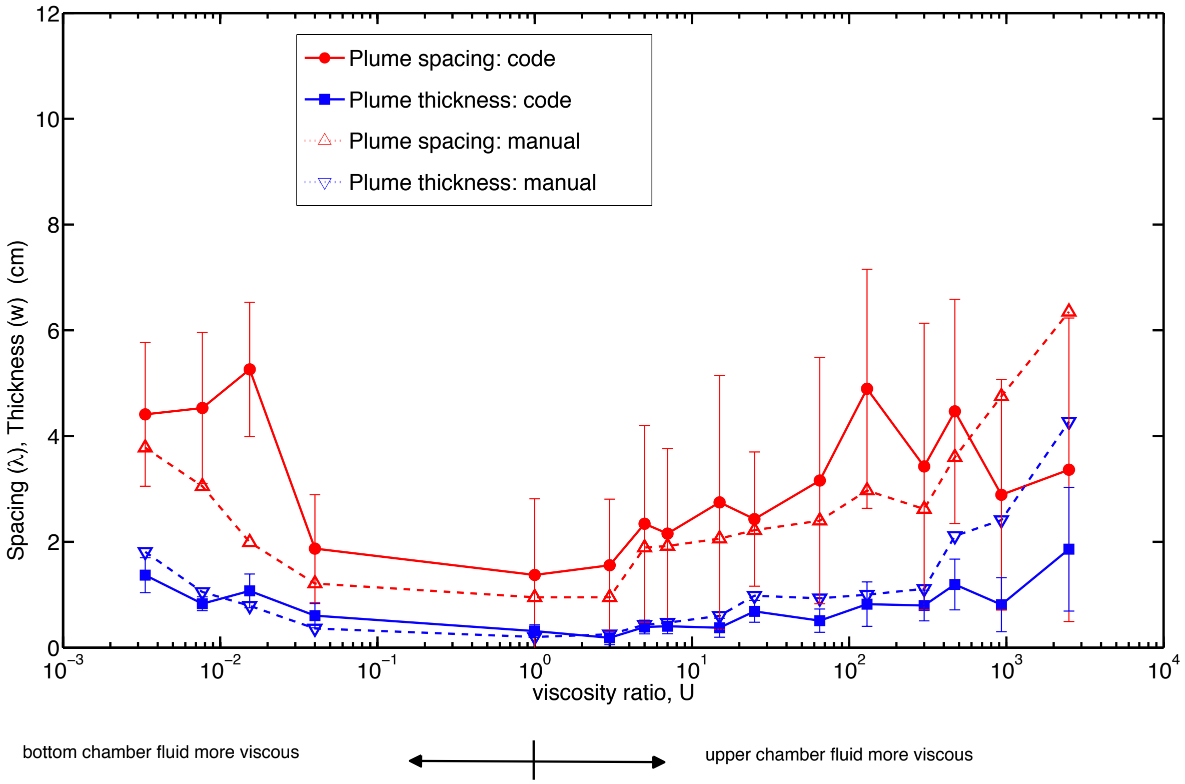


Figure 3: The variation of plume spacing $\lambda$ and thickness $w$ (in cm) with viscosity ratio, $U$. Here, we compare our results obtained from the autocorrelation code and the manual inspection method.

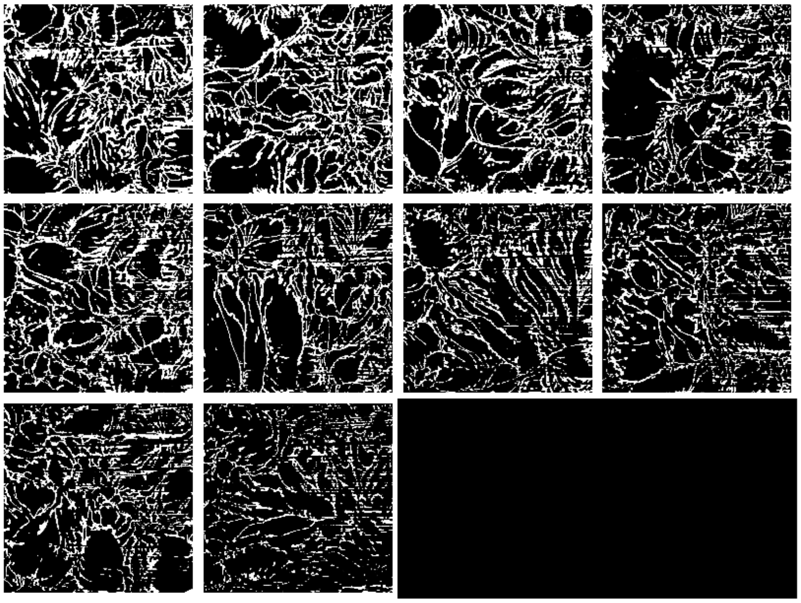

Figure 4: Near-wall planform plume structures showing transient to steady state transitions, for $U = 1$. Images are shown in ascending order of time from start of experiment: t = 42s, 71s, 100s, 129s, 158s, 188s, 217s, 246s, 275s, 305s.

## 2 Transient to steady state transitions in planform plume structures

In order to illustrate the transient to quasi-steady state nature of the convection in our experiments, we have put together a collection of images in Figures 4 to 10 below. Images of the near-wall planforms have been extracted at successive time intervals in each of the experiments with the traverse setup and displayed as a montage.

In Figure 4 ($U = 1$) we see that the structures are almost the same in all the images at different times. However when $U > 1$, the transients take time to settle; In Figures 5, 6, 7, 8 the convection takes time till the fourth frame to settle to a quasi-steady state. When $U < 1$, the cellular patterns become stable only from the fourth frame onwards (Figures 9 and 10). We have selected the fourth frame in each of the cases for the plume spacing analysis.

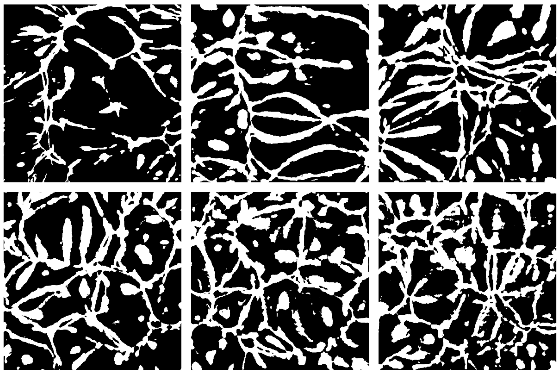

Figure 5: Near-wall planform plume structures showing transient to steady state transitions, for $U = 65$. Images are shown in ascending order of time from start of experiment: t = 46s, 92s, 141s, 190s, 240s, 289s.

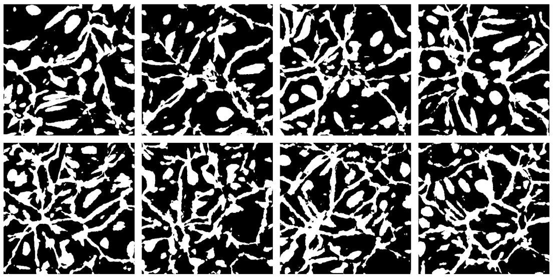

Figure 6: Near-wall planform plume structures showing transient to steady state transitions, for $U = 300$. Images are shown in ascending order of time from start of experiment: t = 35s, 74s, 114s, 154s, 194s, 233s, 273s, 313s.

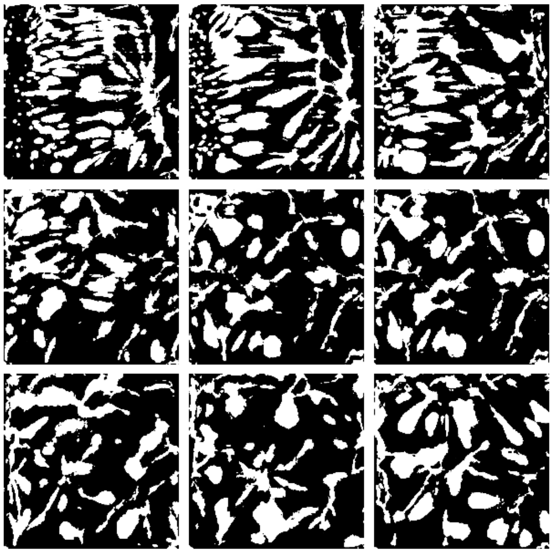

Figure 7: Near-wall planform plume structures showing transient to steady state transitions, for $U = 930$. Images are shown in ascending order of time from start of experiment: t = 126s, 175s, 224s, 273s, 319s, 331s, 380s, 429s, 478s.

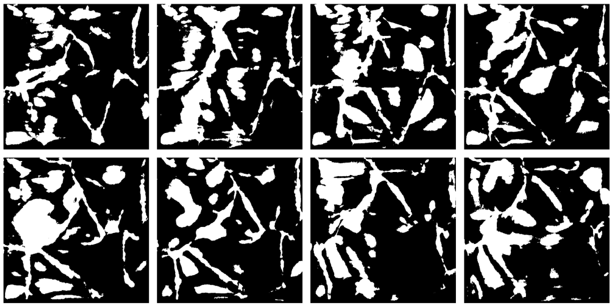

Figure 8: Near-wall planform plume structures showing transient to steady state transitions, for $U = 2500$. Images are shown in ascending order of time from start of experiment: t = 571s, 611s, 651s, 691s, 731s, 771s, 811s, 851s.

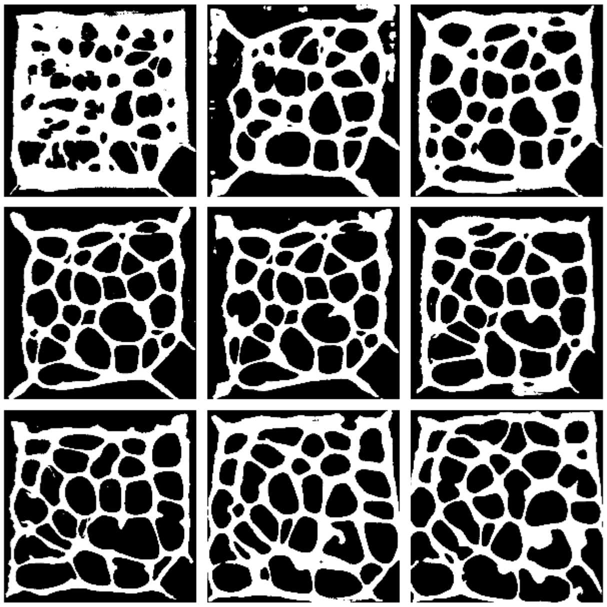

Figure 9: Near-wall planform plume structures showing transient to steady state transitions, for $U = 1/300$. Images are shown in ascending order of time from start of experiment: t = 103s, 154s, 205s, 245s, 254s, 305s, 356s, 407s, 458s.

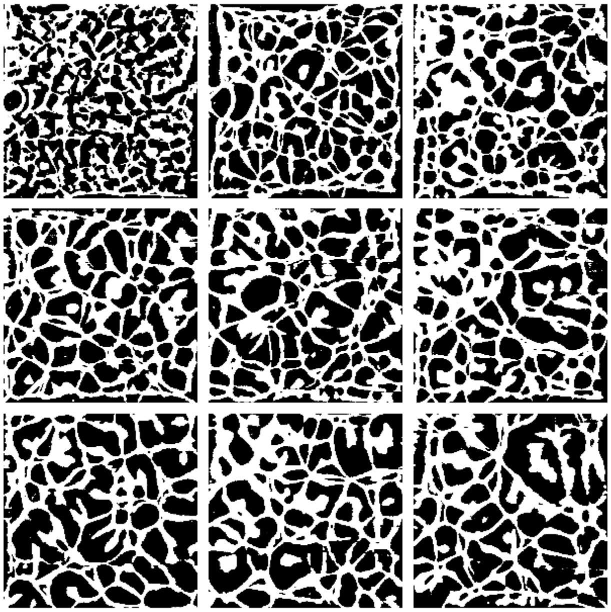

Figure 10: Near-wall planform plume structures showing transient to steady state transitions, for $U = 1/65$. Images are shown in ascending order of time from start of experiment: t = 14s, 63s, 112s, 161s, 210s, 259s, 303s, 352s, 401s.

# 3 Plume dynamics in vertical sections

In the vertical section experiments, we study the effect of $U$ on the plume rise velocities. First, the plume rise was measured by tracking the vertical position of the plume-head over time. From this we obtain the plume height versus time data, an example is shown in Figure 11 for the case $U = 300$.

A second order polynomial was fitted onto this height versus time data, and the velocity was obtained by taking the first derivative. The characteristic velocity for each case of $U$ was taken as the peak in the distribution of plume velocities of all samples and measured heights as shown in Figure 12 for the example cases of $U = 25, 300, 2500$.

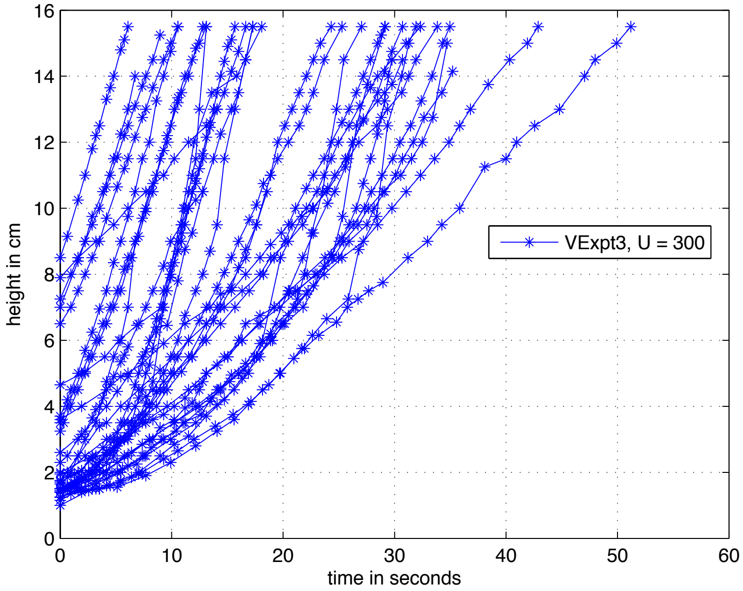


Figure 11: Plume height versus time data samples for $U = 300$.

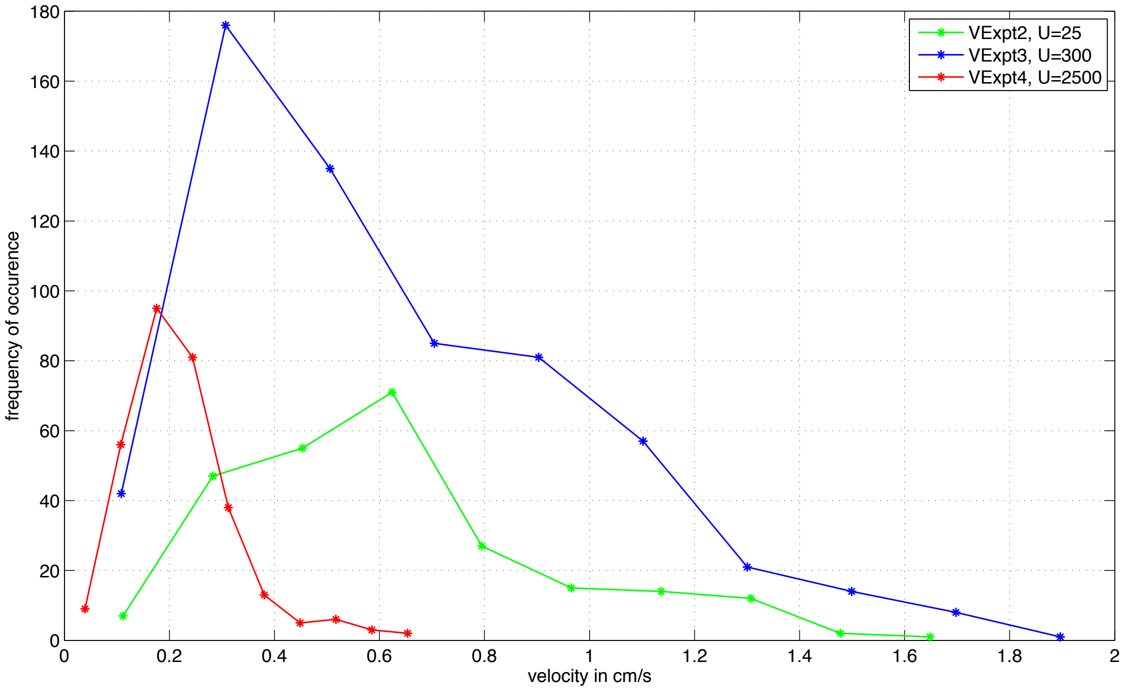


Figure 12: Plume velocity distributions for cases $U = 25, 300, 2500$.

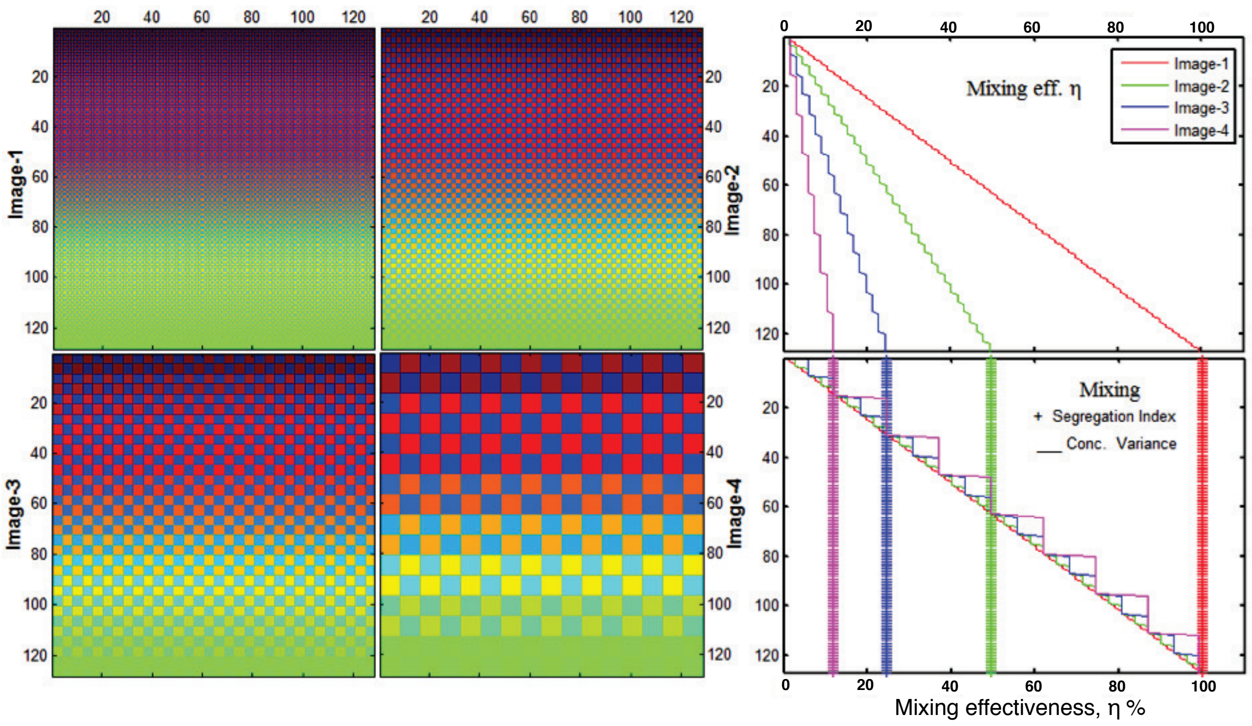


Figure 13: Test of the mixing effectiveness parameter, $\eta$, using synthetic images.

# 4 Mixing effectiveness, $\eta$

The mixing effectiveness, $\eta$ is defined as:

$$\eta = \left[\frac{(\bar{I} - \sigma_I)}{\bar{I}}\right]\left[\frac{N_{cr}}{(N_{max}}\right] \tag{1}$$

As mentioned in section III(C), lower values of $\eta$ indicate poor mixing (either due to high fluctuation in dye concentration or due to large length scale segregation) and higher values of $\eta$ indicate good mixing (in this case, *both* the magnitude of concentration fluctuations and the length scale of segregation are small).

In the set of synthetic images shown in Figure 13, each image has one length scale of segregation and in each image, the intensity of fluctuation increases as we move from the bottom of the image to the top. We also present mixing effectiveness, $\eta$, segregation-index, and concentration variance, which are computed along horizontal lines at various vertical positions. Image-1 has the overall best mixing effectiveness compared to other images. In each image, the mixing effectiveness is highest at the bottom where intensities of fluctuation are lowest. The mixing effectiveness based on the segregation index is independent of vertical position in each image, however, it is highest for Image-1 and lowest for Image-4.

## 5 Plume structures at different heights above the mesh

As mentioned in section III(C), a computer-controlled traverse setup was used to visualize the plume structures at different heights from the mesh. This traverse enabled the controlled and precise movement of a horizontal laser sheet in the vertical direction. This data was used to study the amount of mixing between the plume and ambient fluid for a given $U$ at different heights above the mesh.

Here, we present montage sets (selected sequence of snapshots) from experiments conducted using the traverse setup. The images shown in Figures 14, 15, & 16 correspond to the experiments where $U = 300, 2500$ and $1/300$. The sequence of raw images are spaced 1 second apart in time, and correspond to a change in 3 mm height of traverse. The images start at the near-wall planform structure and proceed to the images acquired when the laser sheet moves up. At half-way through the sequence shown, the traverse reaches the maximum height, and then onwards, all the images correspond to the laser sheet moving downwards. In the end of the sequence, the traverse brings the laser sheet back to the near-wall height once again.

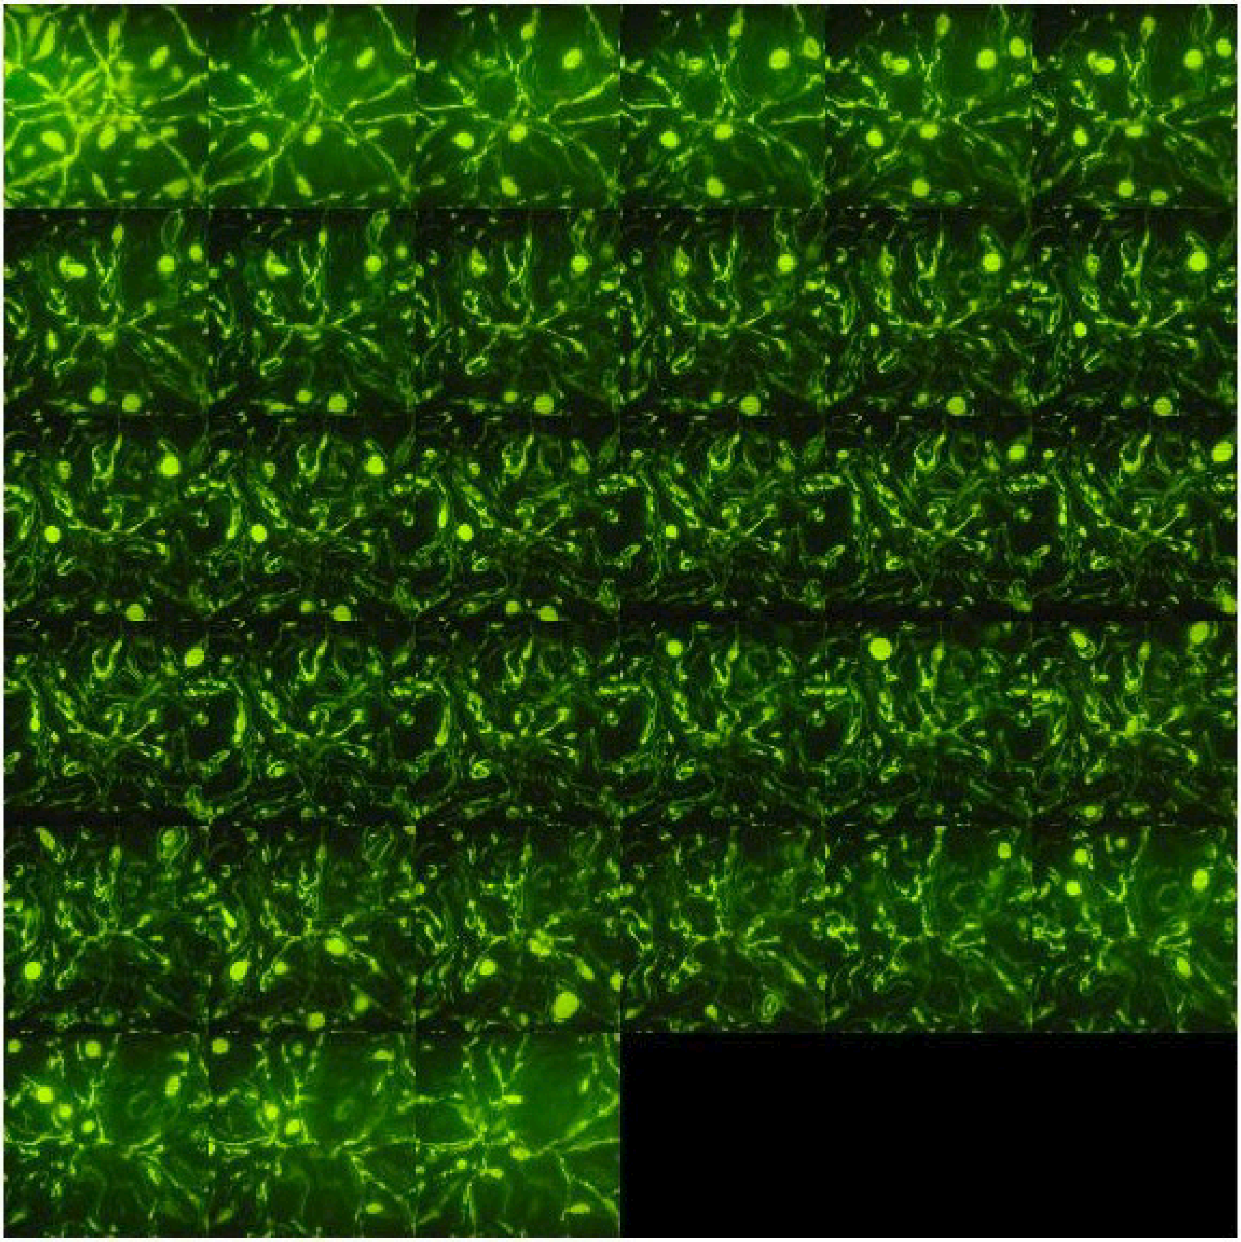

Figure 14: Montage of raw images for the case $U = 300$.

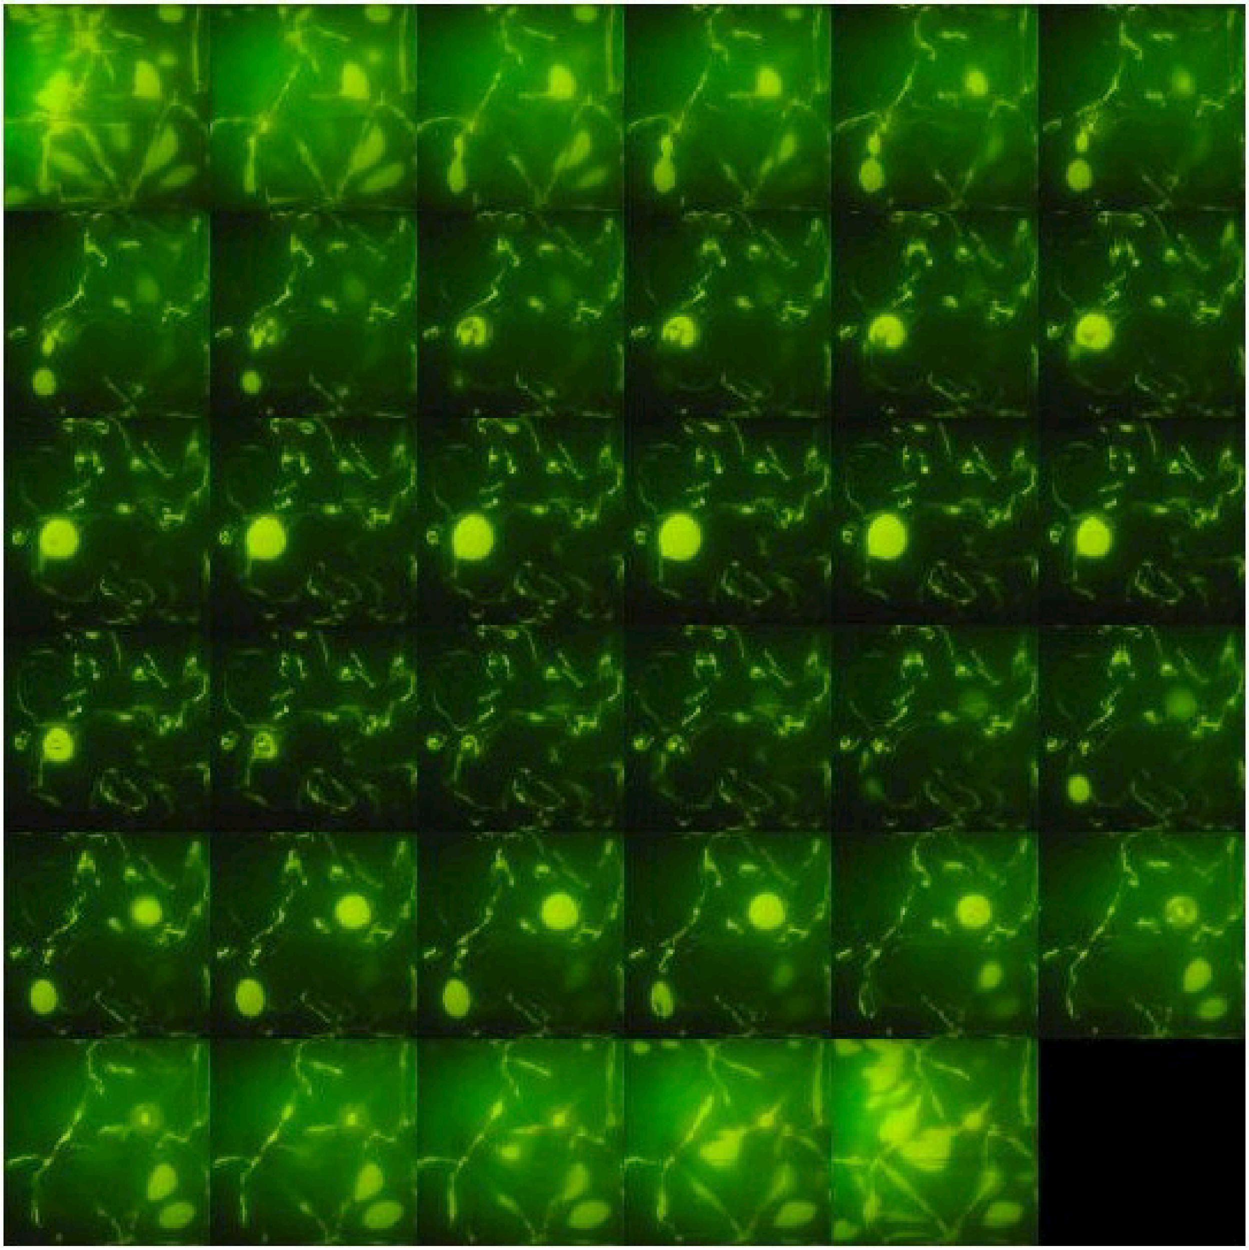

Figure 15: Montage of raw images for the case $U = 2500$.

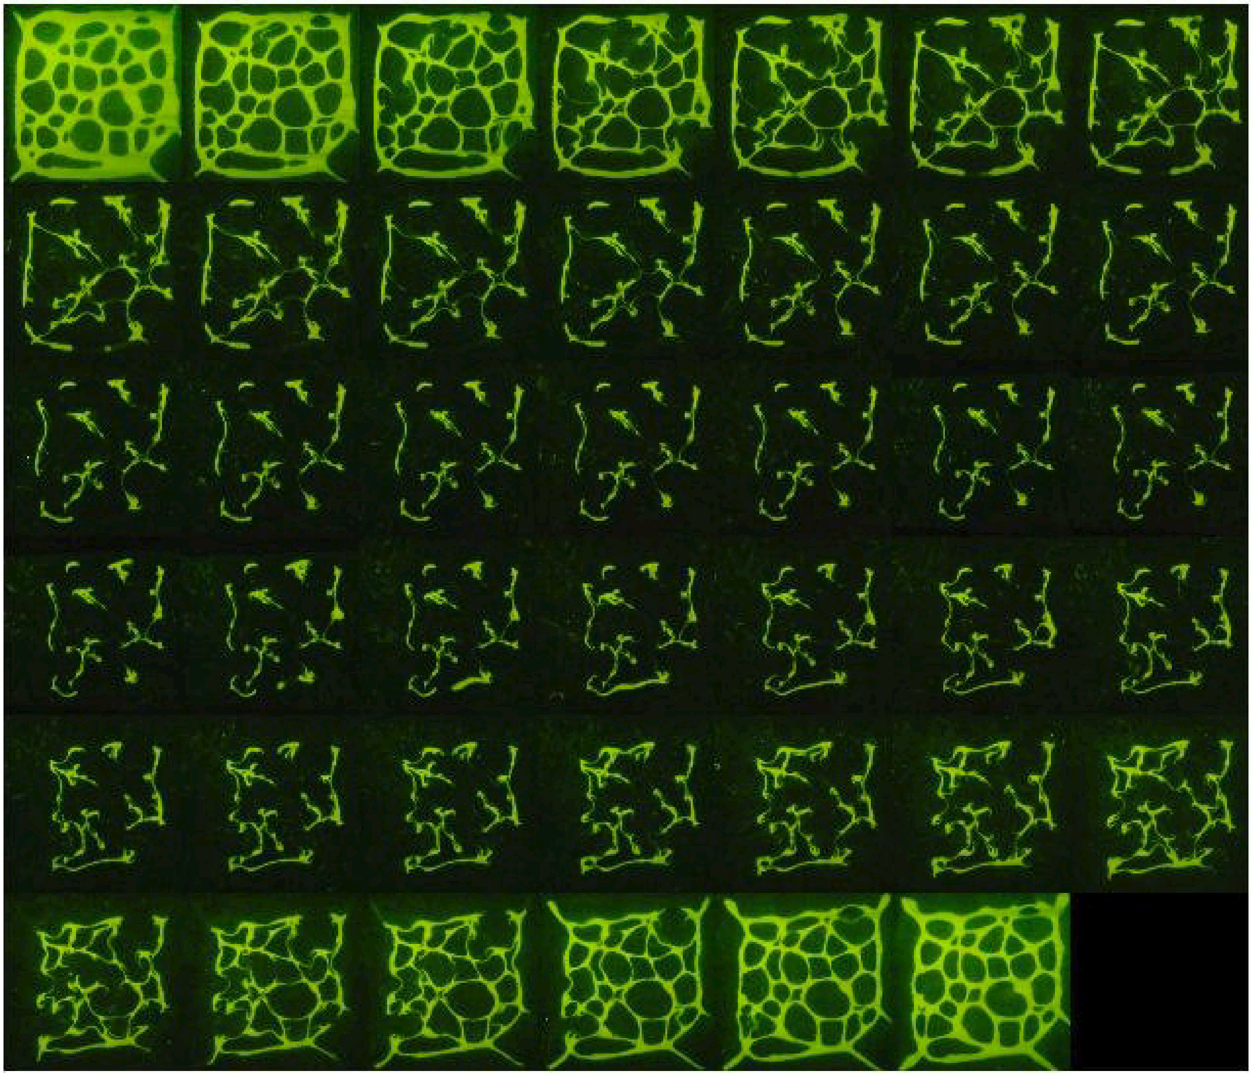

Figure 16: Montage of raw images for the case $U = 1/300$.

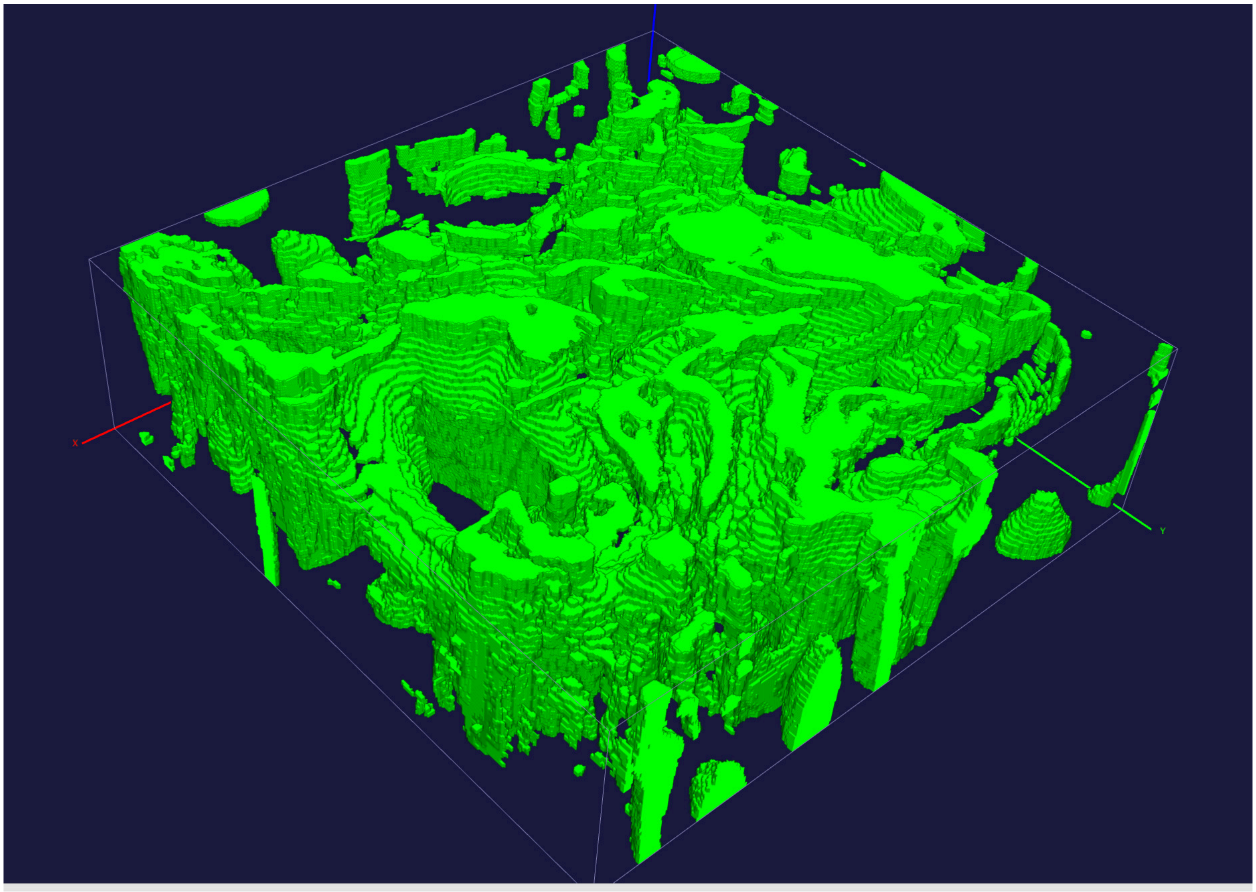

Figure 17: A 3D reconstructed isometric view of the plume structure for $U = 300$.

# 6 Plume morphology in three-dimensions

The images from the traverse experiments (described in the previous section) can be used to reconstruct the plume structure in three-dimensions. This is done by selecting frames at regular intervals and converting the images to binary. The images are basically stacked onto each other in the z axis (height) and stored in a single matrix. The plume data between any two frames are interpolated and the plume surfaces are plotted as iso-surfaces using Tecplot software. Figure 17 shows an example of such a 3-D reconstruction for the case of $U = 300$. This 3-D reconstruction method provides a valuable tool to visualize the plume structure in three-dimensions. Also, the plume structure can be visualized in further detail by moving cross-sections throughout the 3-D reconstruction. The cross-sections can be highlighted and the other regions can be made invisible. The movement of slices in x, y or z direction can be exported into videos.

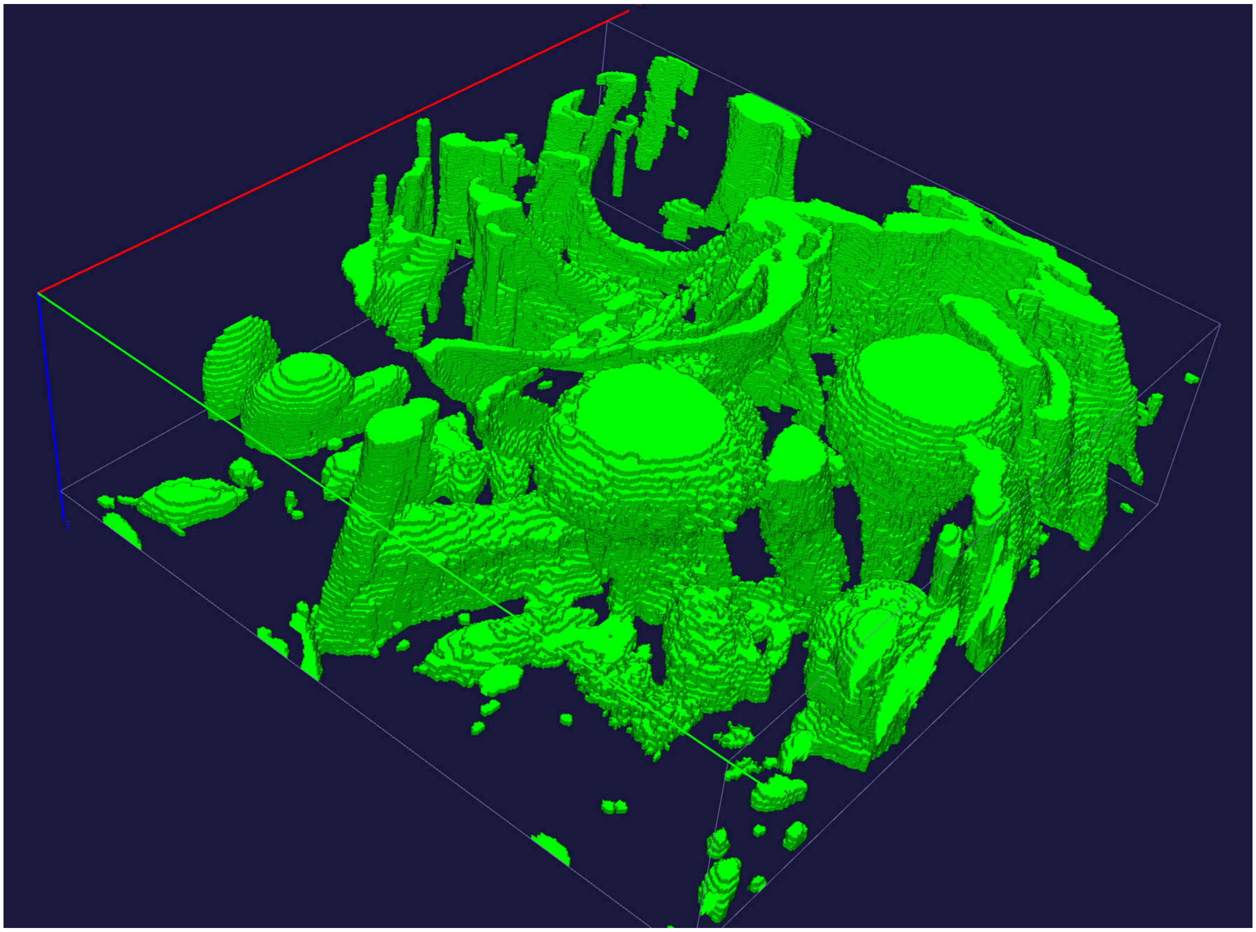

Figure 18: A 3D reconstructed isometric view of the plume structure for $U = 2500$.

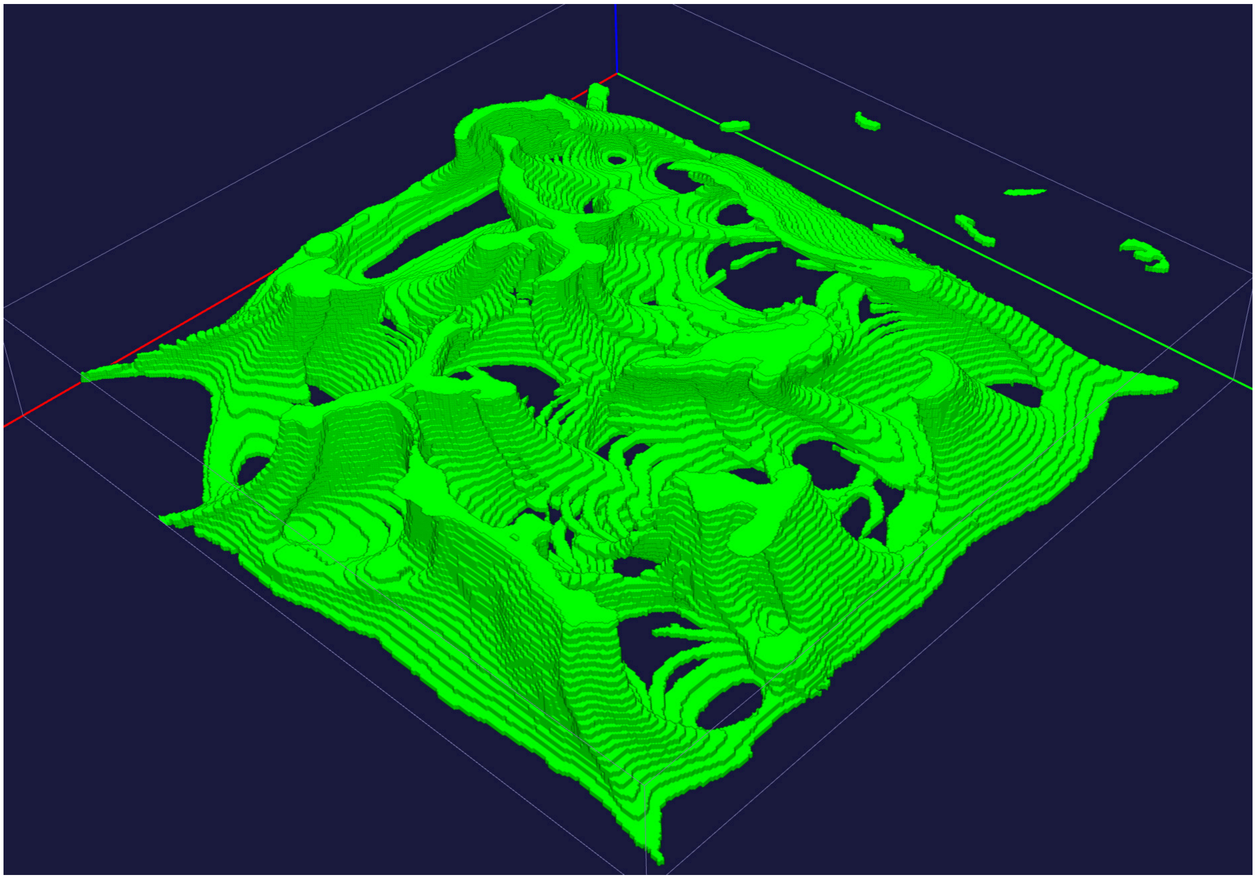

Figure 19: A 3D reconstructed isometric view of the plume structure for $U = 1/300$.
